# Supplementary material for: Towards Deep Encrypted Training: Low-Latency, Memory-Efficient, and High-Throughput Inference for Privacy-Preserving Neural Networks
Source: arXiv:2604.16834 source file (2026-04-18)
Supplement: Supplementary file 1 [file Appendix.tex]

% Input Appendix sections here
